# Supplementary material for: Homological Stability for Spaces of Subsurfaces with Tangential Structure
Source: arXiv:1812.06781 source file (2020-08-31)
Supplement: Supplementary file 1 [file PointedSubsurfaces.tex]

These were spaces of subsurfaces with a fixed boundary condition. Now 
we will speak about pointed subsurfaces. Let $M$ denote a closed 
simply-connected smooth manifold and abbreviate $\Sigma_{g,0}$ by 
$\Sigma_g$. Fix 
$q\in 
\Sigma_{g}$, $p\in M$ and an oriented $2$-plane $A$ in $T_pM$. We 
will consider 
the space
\[
	\Emb_A(\Sigma_{g},M)\coloneqq \{f\in \Emb(\Sigma_g,M)\mid 
	\text{$f(q)=p$ and 
	$Df(T_q\Sigma_g)=A$}\} 
\]
equipped with the $C^\infty$-topology. Let $\Diff_q(\Sigma_{g})$ 
denote the 
subgroup of $\Diff^+(\Sigma_g)$ that fixes $q$. This group acts on 
$\Emb_A(\Sigma_{g},M)$ freely via precomposition and we denote the 
quotient by 
$\mathcal{E}_A^+(\Sigma_{g,b},M)$.
\begin{remark} 
In this pointed case we could replace $M$ by a manifold with boundary 
and 
$\Sigma_g$ by $\Sigma_{g,b}$ and include some boundary condition 
$\delta$ into 
this notation, but we will not bother with this. If one wants to 
include a 
boundary into the pointed case, then all proofs regarding the pointed 
case in 
this paper work verbatim and the same results would hold true.
\end{remark}
